# Supplementary material for: Oscillatory chiral flows in confined active fluids with obstacles
Source: arXiv:2010.14396 source file (2020-10-27)
Supplement: Supplementary file 1 [file Supplementary_Materials.pdf]

# Supplementary Materials for
# Oscillatory chiral flows in confined active fluids with obstacles

Bo Zhang,[1] Benjamin Hilton,[2] Christopher Short,[2] Anton Souslov,[2] and Alexey Snezhko[1,*]

[1] *Materials Science Division, Argonne National Laboratory, 9700 South Cass Avenue, Lemont, IL 60439, USA*

[2] *Department of Physics, University of Bath, Claverton Down, Bath BA2 7AY, UK*

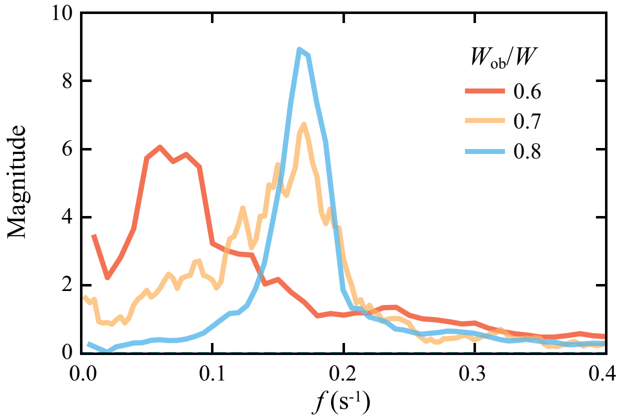


Supplementary Figure 1: **Fast Fourier transform (FFT) of the time evolution of the average tangential velocity as a function of obstacle width.** Average area fractions are $\langle\phi\rangle = 45\phi_c$.

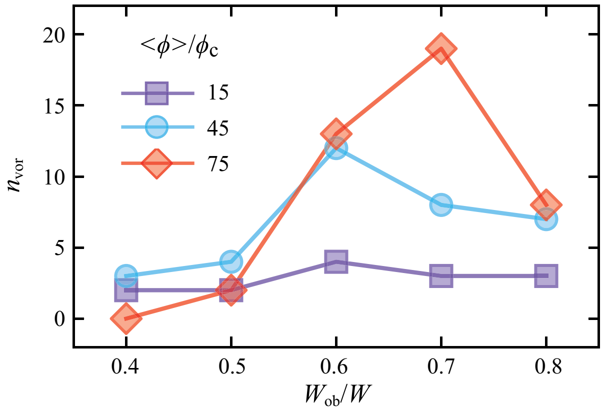


Supplementary Figure 2: **Number of vortices at the vicinity of the obstacle during an obstacle-induced reversal.** The number of vortices $n_{vor}$ is defined at the time when the reversal is about to begin and the number of vortices reaches its maximum. Generally, $n_{vor}$ is low for fast reversals with and high for slow reversals.

## Movies

**Movie 1.** Multiple chirality reversals of active liquids in a track with a rectangular obstacle. The outer diameter of track $D = 2$ mm. The width of the track $W = 0.25$ mm. The width of the obstacle $W_{\text{ob}} = 0.6W$. The area fraction $\langle\phi\rangle = 45\phi_{\text{c}}$. The movie is 4X the real speed.

**Movie 2.** Chirality reversal in a track with a rectangular obstacle. (a) Multiple vortices formed during one chirality reversal of active liquids. $W_{\text{ob}} = 0.6W$. $\langle\phi\rangle = 15\phi_{\text{c}}$. (b) Corresponding velocity (black arrows) and vorticity (background color) fields of active liquids shown in (a). The colormap is same as in Fig. 2c. (c) Corresponding velocity distribution (arrows) of individual rollers in active liquids shown in (a). The velocity arrows are colored based on their direction for better visualization. The colorwheel is same as in Fig. 2d. The outer diameter of track $D = 2$ mm. The width of the track $W = 0.25$ mm. The movie is 0.24X slower than real time.

**Movie 3 (Part 1).** Simulations of chirality reversal induced by rectangular obstacles. These cases demonstrate the two possibilities shown in the phase diagrams for rectangular object chiralities. The left movie shows a case with $W/W_{\text{ob}} = 0.8$ and $\langle\phi\rangle/\phi_{\text{c}} = 20$. In this case, the chirality does not switch when the front hits the obstacle. The right movie shows the case of $W/W_{\text{ob}} = 0.8$ and $\langle\phi\rangle/\phi_{\text{c}} = 10$. This lower density means when the front hits the obstacle, the chirality is reversed.

**Movie 3 (Part 2).** Simulations of hybrid points on phase diagram. The hybrid points on the phase diagram are characterized by the presence of two fronts after impacting the obstacle: one that switches chirality and one that does not. The movie shows this process, visually demonstrating at one point that the two fronts can survive separately even when impacting each other.

**Movie 3 (Part 3).** Phase diagram spike and neighboring points. The spike in the phase diagram that shows a clear non-reversal alongside its two neighbours, demonstrating the origin of the spike feature.

**Movie 3 (Part 4).** Non-stable vortices induced by front reversal. In cases of wide obstacles and high densities (with chirality reversal) vortices can be seen as a result of the shock front interacting with the obstacle. These vortices are visualized with streamline contouring.

**Movie 4.** Formation of apolar state. $W_{\text{ob}} = 0.8W$. $\langle\phi\rangle = 90\phi_{\text{c}}$. The outer diameter of track $D = 2$ mm. The width of the track $W = 0.25$ mm. The movie is 4X the real speed.

**Movie 5 (Part 1).** Active liquids in a track with a triangular obstacle. (a) Active liquid maintains counter clockwise direction. (b) Active liquid reverses the overall flow direction from clockwise to counter clockwise direction. The outer diameter of track $D = 2$ mm. The width of the track $W = 0.25$ mm. $W_{\text{ob}} = 0.6W$. $\langle\phi\rangle = 30\phi_{\text{c}}$. The movie is 2X the real speed.

**Movie 5 (Part 2).** Active liquids in a track with two up triangular obstacles. Particles accumulate at the bottom half of the track due to asymmetric obstacles. The outer diameter of track $D = 2$ mm. The width of the track $W = 0.25$ mm. $W_{\text{ob}} = 0.8W$. $\langle\phi\rangle = 30\phi_{\text{c}}$. The movie is 2X the real speed.

**Movie 6 (Part 1).** Chirality control using a triangular obstacle. The two positions of the triangles are shown simultaneously to demonstrate that the chirality of active fluid flow can be controlled and that steady states can be independent of initial chirality.

**Movie 6 (Part 2).** Density distribution control using two triangular obstacles. This movie demonstrates that the density distribution is no longer uniform when two triangles of the same orientation are induced. In this case, the density is on average higher in the bottom half of the ring than the top.

* Electronic address: `snezhko@anl.gov`
